# Supplementary material for: Role of the ferroelastic strain in the optical absorption of BiVO4
Source: arXiv:2004.10183 ancillary file (2020-07-08)
Supplement: Supplementary file 1 [file main_SI.pdf]

# Role of the ferroelastic strain in the optical absorption of $BiVO_4$ – Supplementary Material

Christina Hill,[1,2] Mads C. Weber,[3] Jannis Lehmann,[3] Tariq Leinen,[3] Manfred Fiebig,[3] Jens Kreisel,[2] and Mael Guennou[2]

[1]*Materials Research and Technology Department, Luxembourg Institute of Science and Technology, 41 rue du Brill, L-4422 Belvaux, Luxembourg*
[2]*Department of Physics and Materials Science, University of Luxembourg, 41 rue du Brill, L-4422 Belvaux, Luxembourg*
[3]*Department of Materials, ETH Zurich, Vladimir-Prelog-Weg 4, 8093 Zurich, Switzerland*

## CONTENTS

I. Definitions of the absorption edge 2
A. Inflexion point of the transmittance curve 2
B. Constant threshold 3
C. Tauc plot 4

II. Positioning of the (001)-oriented sample – anisotropy in the monoclinic plane 5

III. Calculation of the thermal expansion 5

IV. Fit of low-temperature data and extrapolation to 0 K 6

References 8

## I. DEFINITIONS OF THE ABSORPTION EDGE

Different analytical methods exist to define and determine the absorption edge from optical measurements. Here we compare different options, with the aim to show that our conclusions expressed in the main paper do not depend on the choice of a particular method. For simplicity, we neglect here the small non-linearities in the evolution of the absorption edge in the low-symmetry phase.

### A. Inflexion point of the transmittance curve

In the main paper, we defined the absorption edge as the inflexion point of the transmittance curve. The inflexion point was found by fitting the first derivative of the transmittance curve with an asymmetric Gaussian. Fig. 1 shows the temperature dependence of the absorption edge for the (110)-oriented and the (001)-oriented sample. The data were fitted with linear functions, with separate fits below and above $T_{\mathrm{c}}$, and extrapolated to 0 K.

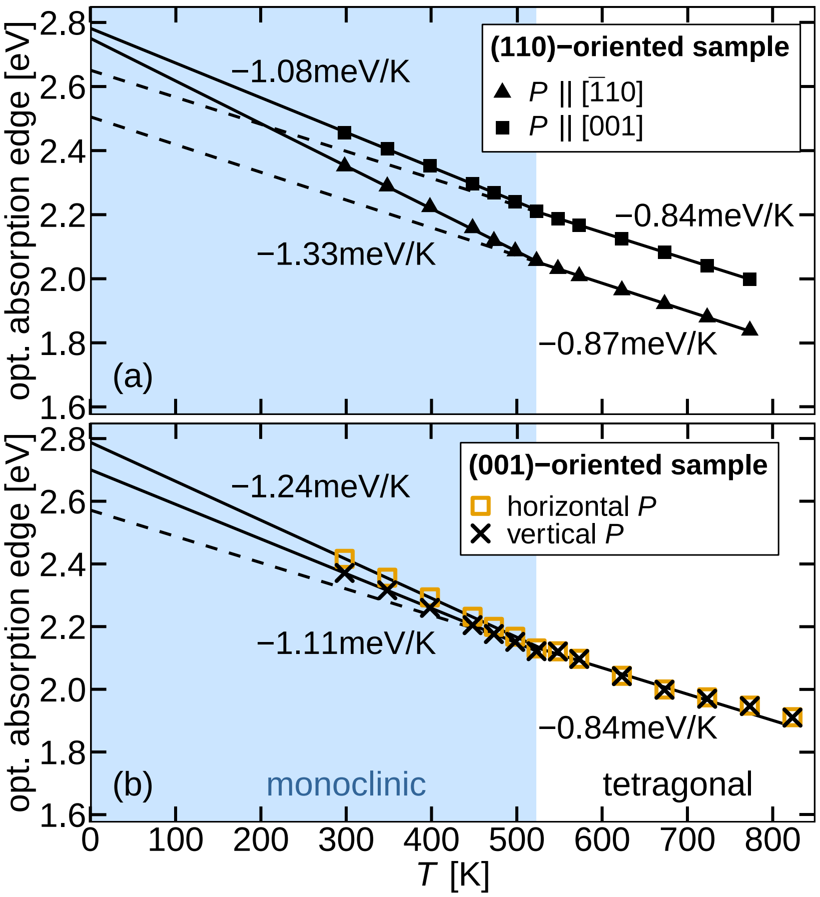


Figure 1: Temperature dependence of the optical absorption edge for (a) the (110)-oriented and (b) the (001)-oriented sample. The absorption edges are extracted as the inflexion point of the transmittance spectra.

### B. Constant threshold

Another way to define an absorption edge is to use the energy corresponding to a fixed - and arbitrary - threshold in transmittance, as it is done for example in Ref. [2]. The drawback of this method is that the extracted value depends on the sample thickness. Here, we show in Fig. 2 the absorption edge deduced at a transmittance value of 1 % for the (110)-oriented sample and the (001)-oriented sample as a function of temperature.

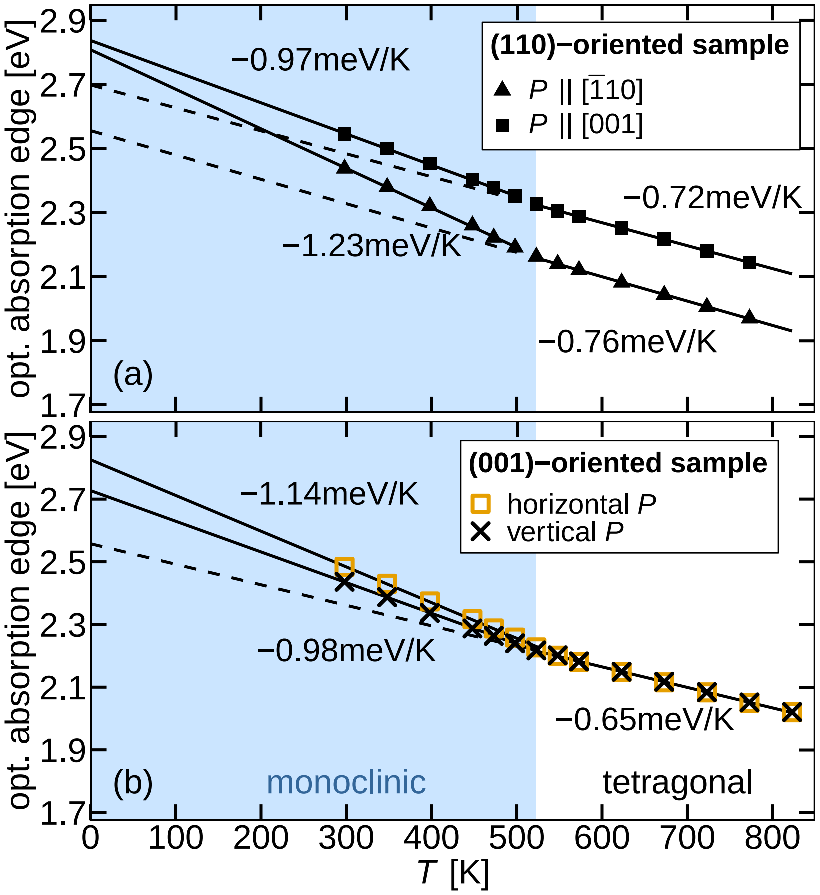


Figure 2: Temperature dependence of the optical absorption edge for (a) the (110)-oriented and (b) the (001)-oriented sample: The absorption edge is deduced at a transmittance value of 1 %.

### C. Tauc plot

Finally, we give the values obtained by making use of the so-called Tauc plot. The method is based on the theory of interband optical absorption. As discussed in the main paper, knowledge about the nature of the involved interband optical absorption is required. Fig. 3 shows the absorption edge deduced from the Tauc plot assuming an indirect band-to-band transition for both samples as a function of temperature. The Tauc plots for the (110)-oriented sample are shown in the main paper.

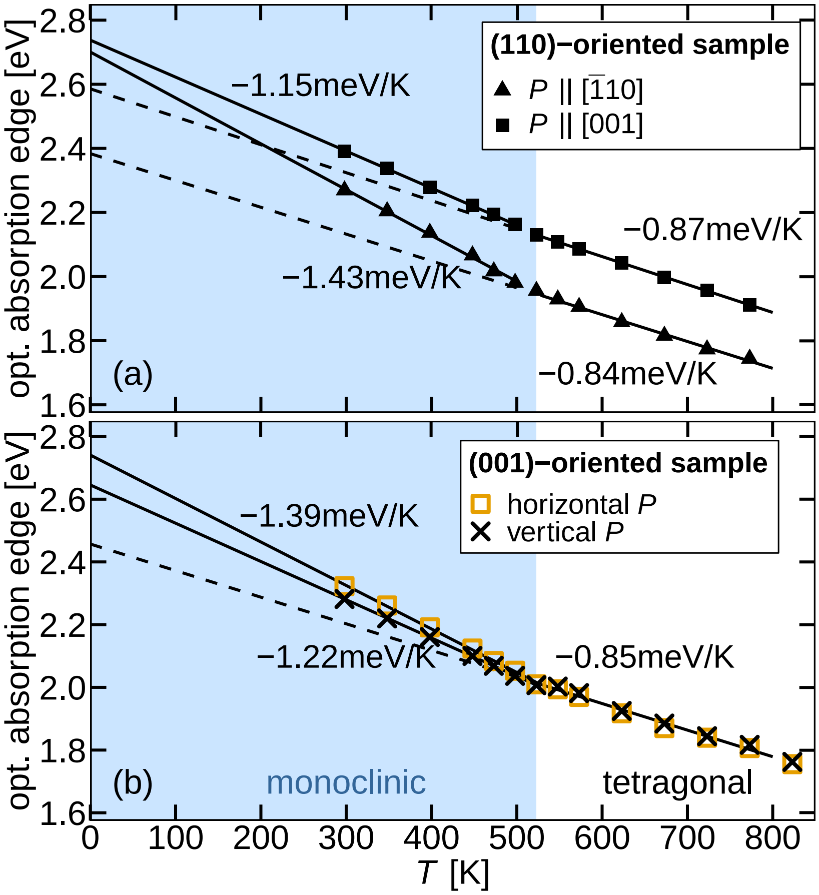


Figure 3: Temperature-dependence of the optical absorption for (a) the (110)-oriented sample and (b) the (001)-oriented sample: The absorption edge is extracted from the Tauc plot assuming an indirect transition.

In all cases, the main conclusions are identical: the tetragonal phase exhibits the same anisotropy, the influence of the phase transition is clearly seen as a kink, and the fundamental absorption edge is found for light polarized perpendicular to the principal axis. The insignificant differences are an offset of the absolute values, and some changes in the values for the slopes.

## II. POSITIONING OF THE (001)-ORIENTED SAMPLE – ANISOTROPY IN THE MONOCLINIC PLANE

In the monoclinic phase, optical anisotropy is expected in the plane perpendicular to the principal axis. In order to estimate the amplitude of the anisotropy, we performed an experiment at fixed wavelength of 515 nm and at room temperature on the (001)-oriented sample. We chose 515 nm because it is close to the absorption edge and therefore we expected significant difference in transmittance for different polarization directions. Fig. 4 shows the transmittance at 515 nm as a function of polarization direction $P$. The sample was aligned in such a way that the maximum transmittance occurred close to the horizontal $P$ and the minimum at vertical $P$. The position of the sample is shown in the inset of Fig. 4. The evolution of the transmittance is fitted with a sinusoidal function.

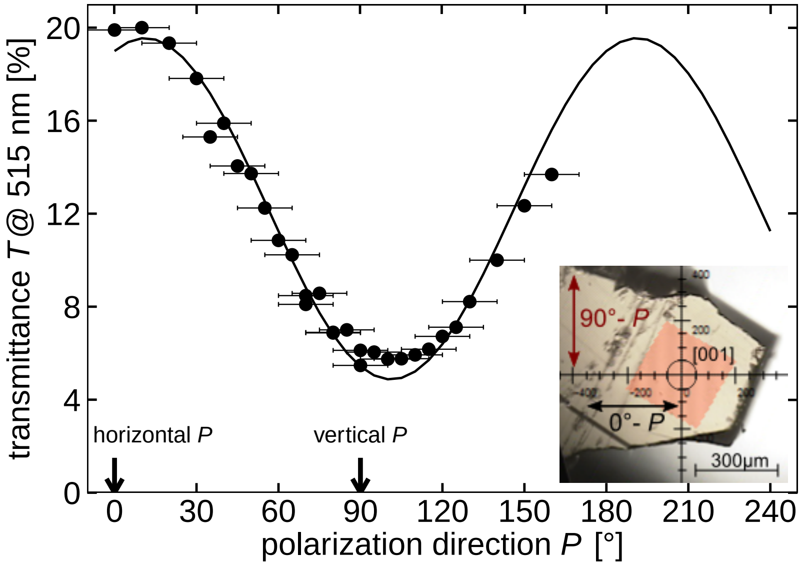


Figure 4: Transmittance as a function of polarization direction, measured at a fixed wavelength of 515 nm and at room temperature on the (001)-oriented sample.

## III. CALCULATION OF THE THERMAL EXPANSION

The definition for the volumetric thermal expansion coefficient is given by:

$$\alpha = \frac{1}{V}\frac{\mathrm{d}V}{\mathrm{d}T}$$

We can directly estimate this coefficient for the tetragonal and monoclinic phases of $BiVO_4$ using the experimental data from Ref. [1]. In both phases, the volume can be considered to change linearly with temperature. We therefore assume linear trends above and below $T_\mathrm{c}$

$$\alpha^{\mathrm{mono}} = \frac{1}{V_0}\left.\frac{\mathrm{d}V}{\mathrm{d}T}\right|_{\mathrm{mono}} = 1.4\times10^{-5}\,\mathrm{K}^{-1} \quad \text{and} \quad \alpha^{\mathrm{tetra}} = \frac{1}{V_0}\left.\frac{\mathrm{d}V}{\mathrm{d}T}\right|_{\mathrm{tetra}} = 4.7\times10^{-5}\,\mathrm{K}^{-1} \tag{1a}$$

where $V_0 = 310.1\,\mathrm{\AA}^3$ is the volume at $T_\mathrm{c}$. In doing so, we neglect the temperature dependence of the thermal expansion, but the error made is not larger than 1%, which is perfectly acceptable for our purpose.

We can also take into account the anisotropy of the thermal expansion and describe it by a second-rank tensor. In the tetragonal symmetry, the tensor has two independent coefficients $\alpha_{11}^{\mathrm{tetra}}$ and $\alpha_{33}^{\mathrm{tetra}}$. With the same approach as before, and linear fits to the evolution of $a$ and $c$ above $T_\mathrm{c}$, we can write

$$\alpha_{33}^{\mathrm{tetra}} = \frac{1}{c_0}\left.\frac{\mathrm{d}c}{\mathrm{d}T}\right|_{\mathrm{tetra}} = 2.08\times10^{-5}\,\mathrm{K}^{-1} \quad \text{and} \quad \alpha_{11}^{\mathrm{tetra}} = \frac{1}{a_0}\left.\frac{\mathrm{d}a}{\mathrm{d}T}\right|_{\mathrm{tetra}} = 1.36\times10^{-5}\,\mathrm{K}^{-1} \tag{1b}$$

where $a_0$ and $c_0$ are again the values at $T_c$. These values can be directly compared to the evolution of the secondary strain coefficients in the monoclinic phase, denoted as $\varepsilon_{11}^{SS}$ and $\varepsilon_{33}^{SS}$ in Ref. [1]. These also behave almost linearly with temperature and we have

$$\frac{d\varepsilon_{33}^{SS}}{dT} = -1.45 \times 10^{-5}\,\mathrm{K}^{-1} \quad \text{and} \quad \frac{d\varepsilon_{11}^{SS}}{dT} = -1.03 \times 10^{-5}\,\mathrm{K}^{-1} \tag{1c}$$

The negative sign expresses the fact that these strains act against the background thermal expansion. More importantly, the ratios $(\varepsilon_{33}^{SS}/\varepsilon_{11}^{SS})$ and $(\alpha_{33}^{tetra}/\alpha_{11}^{tetra})$ are very similar, which justifies the use of a single coefficient to compare the thermal expansions in the two phases, and finally our estimation of its contribution to the shift of the optical absorption edge.

## IV. FIT OF LOW-TEMPERATURE DATA AND EXTRAPOLATION TO 0 K

In the tetragonal high-temperature phase, the absorption edge as a function of temperature is well described by a linear fit. However, at low temperatures the evolution of the absorption edge is expected to deviate from linearity. A first cause of non-linearity is the dependence on spontaneous strain. As described in the main text, we describe this by a power-law

$$\Delta E_{opt} = A(T_c - T)^{\beta}$$

derived from Landau theory, where $T_c$ is the critical temperature and $A$, $\beta$ are fitting constants. For the fitting, $T_c$ has been fixed to 523 K corresponding to the phase transition temperature of $BiVO_4$.

In addition, other causes of non-linearly can be expected.[4] To describe the saturation at low temperatures $T$, we fitted the experimental data in the monoclinic phase with different functions. Since we lack data at low temperatures, we could not reasonably fit all parameters. Instead we use here physical arguments to estimate and fix some of the required parameters.

First, we consider the Varshni function, an empirical function often used for classical semiconductors

$$E_g(T) = E_g(0) - \alpha T^2/(T + T_0)$$

where $E_g$ is the direct or indirect band gap, $E_g(0)$ the band gap at 0 K and $\alpha$ the Varshni coefficient.[5] The parameter $T_0$ defines the temperature range over which the function saturates at low temperatures, and is found to be of the order of the Debye temperature $\Theta_D$.[3] Here, we simply assume that $T_0$ is equal to $\Theta_D$. Considering the highest vibrational mode in $BiVO_4$ of 830 $cm^{-1}$, the Debye temperature is estimated to be 1200 K.

Second, we consider the Bose-Einstein function that takes into account the electron-phonon interaction

$$E_g(T) = E_g(0) - \frac{2a_B}{\exp(\Theta_E/T) - 1}$$

where $a_B$ is a measure for the electron-phonon coupling in the crystal and $\Theta_E$ is the average temperature of the phonon interaction[3] and marks the temperature range where $E_g$ saturates. Following the comparison shown in Ref. [3], we fixed $\Theta_E$ to 900 K from the following relation $\Theta_D = 4\Theta_E/3$.

Fig. 5 shows the absorption edge deduced from the Tauc plot assuming an indirect band gap for $P \parallel [\bar{1}10]$ in the monoclinic phase, which is the fundamental absorption edge. The extrapolations are shown for each of the functions described above, and the values at 0 K are shown in Table I. We conclude that the low-temperature effects could lead to a lowering of the band-gap value by as much as 0.3 eV.

Table I: Fundamental absorption edge at 0 K obtained by extrapolation with different fitting functions.

| Fitting function | $E_{opt}$ [eV] @ $T = 0\,K$ |
|---|---|
| linear fit | 2.70 |
| power-law fit | 2.62 |
| Varshni fit | 2.47 |
| Bose-Einstein fit | 2.37 |

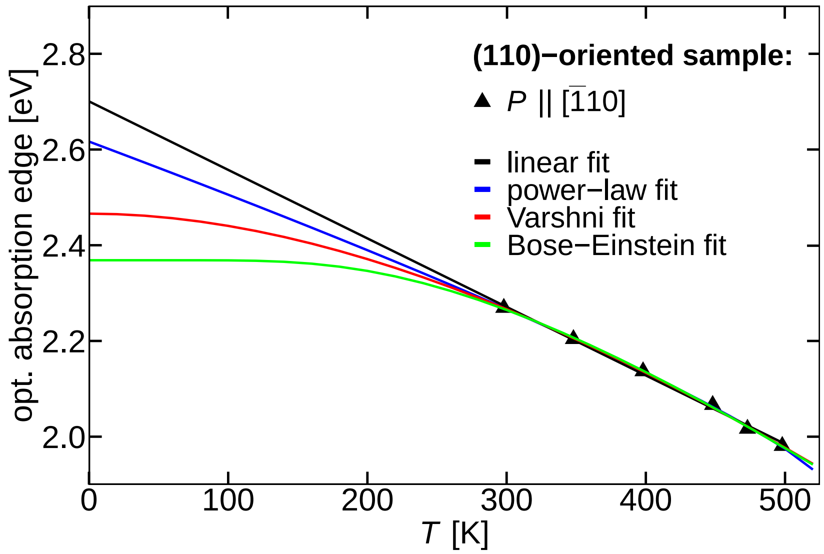


Figure 5: Optical absorption edge in the monoclinic low-temperature phase measured on the (110)-oriented sample, with extrapolations down to 0 K.

[1] W. I. F. David and I. G. Wood. Ferroelastic phase transition in $BiVO_4$ : V. Temperature dependence of $Bi^{3+}$ displacement and spontaneous strains. *Journal of Physics C: Solid State Physics*, 16(26):5127–5148, September 1983.

[2] W. Heiss, R. Kirchschlager, G. Springholz, Z. Chen, M. Debnath, and Y. Oka. Magnetic polaron induced near-band-gap luminescence in epitaxial EuTe. *Physical Review B*, 70(3):035209, July 2004.

[3] Biljana Pejova, Bahattin Abay, and Irina Bineva. Temperature dependence of the band-gap energy and sub-band-gap absorption tails in strongly quantized znse nanocrystals deposited as thin films. *The Journal of Physical Chemistry C*, 114(36):15280–15291, September 2010.

[4] I. A. Vainshtein, A. F. Zatsepin, and V. S. Kortov. Applicability of the empirical Varshni relation for the temperature dependence of the width of the band gap. *Physics of the Solid State*, 41(6):905–908, 1999.

[5] Y. P. Varshni. Temperature dependence of the energy gap in semiconductors. *Physica*, 34:149–154, 1967.
